# Supplementary material for: The Counterfeit Conundrum: Can Code Language Models Grasp the Nuances of Their Incorrect Generations?
Source: arXiv:2402.19475 source file (2024-02-29)
Supplement: Supplementary file 1 [file appendix-results-later.tex]

% \subsection{ROC}
% \begin{figure*}[ht]
%     \centering
%     \begin{subfigure}[b]{0.75\textwidth}
%         \centering
%         \includegraphics[width=\linewidth]{figures/roc/humaneval_all.pdf}
%         \subcaption{HumanEval ROC Curves}
%     \end{subfigure}
%     \vfill
%     \begin{subfigure}[b]{0.99\textwidth}
%         \centering
%         \includegraphics[width=\linewidth]{figures/roc/livecodebench_all.pdf}
%         \subcaption{LeetCode ROC Curves}
%     \end{subfigure}
%     \hfill
% \end{figure*}

% \begin{figure}[ht]
% \ContinuedFloat
%     \centering
%     \begin{subfigure}[b]{0.75\textwidth}
%         \centering
%         \includegraphics[width=\linewidth]{figures/roc/odex_all.pdf}
%         \subcaption{ODEX ROC Curves}
%     \end{subfigure}
%     \caption{ROC curves for correctness prediction with and without CoT.}
% \end{figure}

% \subsection{Violin Plots}
% \begin{figure*}[ht]
%     \centering
%     \begin{subfigure}[b]{0.49\textwidth}
%         \centering
%         \includegraphics[width=\linewidth]{figures/prediction_distribution/violin_humaneval_codellama-34b.pdf}
%         \subcaption{HumanEval (CL-34B)}
%     \end{subfigure}
%     \hfill
%     \begin{subfigure}[b]{0.49\textwidth}
%         \centering
%         \includegraphics[width=\linewidth]{figures/prediction_distribution/violin_humaneval_deepseek-instruct-33b.pdf}
%         \subcaption{HumanEval (DS-I-33B)}
%     \end{subfigure}
%     \begin{subfigure}[b]{0.49\textwidth}
%         \centering
%         \includegraphics[width=\linewidth]{figures/prediction_distribution/violin_livecodebench_deepseek-instruct-6.7b.pdf}
%         \subcaption{LeetCode (DS-I-6.7B)}
%     \end{subfigure}
%     \hfill
%     \begin{subfigure}[b]{0.49\textwidth}
%         \centering
%         \includegraphics[width=\linewidth]{figures/prediction_distribution/violin_livecodebench_deepseek-instruct-6.7b.pdf}
%         \subcaption{LeetCode (DS-I-33B)}
%     \end{subfigure}    
%     \hfill
%     \begin{subfigure}[b]{0.49\textwidth}
%         \centering
%         \includegraphics[width=\linewidth]{figures/prediction_distribution/violin_odex_starcoder.pdf}
%         \subcaption{ODEX (StarCoder)}
%     \end{subfigure}    
%     \hfill
%     \begin{subfigure}[b]{0.49\textwidth}
%         \centering
%         \includegraphics[width=\linewidth]{figures/prediction_distribution/violin_odex_codellama-34b.pdf}
%         \subcaption{ODEX (CL-34B)}
%     \end{subfigure}    
%     \caption{Distribution of probabilities}
% \end{figure*}
